# Supplementary material for: An Empirical Study on Finding Spans
Source: arXiv:2210.06824 source file (2022-10-14)
Supplement: Supplementary file 1 [file dataset_stats.tex]

\subsection{ACE Statistics}
\begin{table}[h]
\resizebox{\linewidth}{!}{%
    \centering
    \begin{tabular}{lcccccc}
      \toprule
         & \multicolumn{3}{c}{ACE05-R} & \multicolumn{3}{c}{ACE05-E\textsuperscript{+}} \\
         \cmidrule(lr){2-4}\cmidrule(lr){5-7}
         & Train & Dev & Test & Train & Dev & Test \\
      \midrule
      \#Instances & 8486 & 2031 & 1733 & 19181 & 901 & 676 \\
      \#Entities & 26470 & 6402 & 5476 & 47452 & 3423 & 3673 \\
      \#Relations & 4781 & 1177 & 1149 & 7154 & 728 & 802 \\
      \#Events & - & - & - & 4419 & 468 & 424 \\
      \bottomrule
    \end{tabular}
    }
    \caption{Summary statistics for ACE05 dataset}
    \label{tab:ace_stats}
\end{table}

\subsection{SQuAD 2.0 Statistics}
\begin{table}[h]
    \centering
    \resizebox{0.6\linewidth}{!}{%
    \begin{tabular}{l|cc}
      \toprule
         & Train &Dev \\
      \midrule
         \#Answerable & 86821 & 5928 \\
         \#Unanswerable & 43498 & 5945 \\
      \bottomrule
    \end{tabular}
    }
    \caption{Summary stats for the SQuAD2.0 dataset.}
    \label{tab:SQuAD_stats}
\end{table}
