# Supplementary material for: An Empirical Study on Finding Spans
Source: arXiv:2210.06824 source file (2022-10-14)
Supplement: Supplementary file 2 [file detailed_setup.tex]

\paragraph{EE, RE, and NER}

%Reason to use OneIE over DYGIE, I am not sure whether this is the correct place that I should place this
%We chose OneIE as our baseline for NER, RE, and EE because that it is well-known to the IE community and it is a strong baseline for these tasks with open source access. In addition, compared to other SoTA models that jointly train the span finding module via the downstream modules like DYGIE, OneIE trains the span finding module only with the objective of span extraction, which provides the flexibility to better serve our purpose of only replacing the span finding module without introducing modifications to other components.

\paragraph{Coreference Resolution}

\paragraph{Question Answering}
