# Supplementary material for: An Empirical Study on Finding Spans
Source: arXiv:2210.06824 source file (2022-10-14)
Supplement: Supplementary file 3 [file full_experiments.tex]

% \paragraph{SQuAD 2.0 Results}
% \begin{table}[h]
% \resizebox{\linewidth}{!}{%
%     \centering
%     \begin{tabular}{l|cc}
%       \toprule
%         \bf Approach & \bf EM & \bf F\textsubscript{1}\\
%       \midrule
%         CRF(RoBERTa\textsubscript{base}) & 74.4  & 80.8\\
%         +BiLSTM & 74.7 & 81.3\\
%         CRF(T5\textsubscript{base}) & 58.1  & 67.3\\
%         +BiLSTM & 62.1 & 70.7\\
%       \midrule
%         Boundary Prediction(RoBERTa\textsubscript{base}) &77.6 & 85.0\\
%         +BiLSTM & 78.1 & 85.4\\
%         Boundary Prediction(T5\textsubscript{base}) &70.3 &76.1\\
%         +BiLSTM & 73.9 & 79.9\\
%       \midrule
%         Span Enumeration(RoBERTa\textsubscript{base}) &68.8 &73.8\\
%         +BiLSTM & 68.7 & 73.9\\
%         Span Enumeration(T5\textsubscript{base}) & 62.3 & 66.1\\
%         +BiLSTM & 63.6 & 67.1\\
%       \bottomrule
%     \end{tabular}
%     }
%     \caption{Full experiment results on SQuAD 2.0 dev set.}
%     \label{tab:qa_exps}
% \end{table}

%\begin{table*}[h]
% \resizebox{\textwidth}{!}{%
%     \centering
%     \begin{tabular}{l|cccccccccccccccc}
%       \toprule
%         \bf Approach & \multicolumn{3}{c}{\bf Macro} & \multicolumn{3}{c}{\bf MUC} & \multicolumn{3}{c}{\bf B\textsuperscript{3}}& \multicolumn{3}{c}{\bf CEAF} & \multicolumn{3}{c}{\bf Mention} \\
%         \cmidrule(lr){2-4}\cmidrule(lr){5-7}\cmidrule(lr){8-10}\cmidrule(lr){11-13}\cmidrule(lr){14-16}
%          & Prec & Rec & \bf F\textsubscript{1}& Prec & Rec & \bf F\textsubscript{1}& Prec & Rec & \bf F\textsubscript{1} & Prec & Rec & \bf F\textsubscript{1}& Prec & Rec & \bf F\textsubscript{1}& \\
%       \midrule
%         CRF(RoBERTa\textsubscript{base}) &63.2&	48.1&	54.0&	72.8&	63.2&	67.7&	56.3&	49.3&	52.6&	60.4&	31.8&	41.6&	80.1&	73.7&	76.8 \\
%         +BiLSTM &63.6&	48.4&	54.2&	73.2&	63.5&	68.0	&56.3&	50.0&	53.0&	61.4&	31.6&	41.7	&81.2	&73.3	&77.0  \\
%         -Overlap &63.0&	49.4&	54.5&	72.5&	64.6&	68.3&	54.5&	51.4&	52.9&	61.9	&32.1&	42.3&	81.7	&72.8&	77.0  \\
%         -Overlap+BiLSTM &61.8&	52.0&	55.4	&70.5&	67.4&	68.9&	52.7&	55.4&	54.0	&62.3&	33.3	&43.4&	79.3	&75.6	&77.4   \\

%         CRF(T5\textsubscript{base}) &66.6	&59.2&	62.3&	72.8&	70.0	&71.4&	59.9&	60.1&	60.0&	67.1&	47.4&	55.6&	78.5&	76.3&	77.4  \\
%         +BiLSTM &60.4	&51.9&	54.7&	69.4&	67.2&	68.3	&50.9&	55.7	&53.2	&60.7&	32.7&	42.5&	78.8&	75.7&	77.2\\
%         -Overlap &61.3&	52.1&	55.1&	70.4&	67.7&	69.0&	51.5&	56.2&	53.7&	62.0&	32.3&	42.5&	79.4	&76.0&	77.7\\
%         -Overlap+BiLSTM &66.1&	48.0&	55.2&	75.6&	62.3	&68.3&	61.5&	47.5&	53.6&	61.2&	34.0&	43.8&	80.9&	73.2&	76.8\\

%       \midrule
%         Boundary(RoBERTa\textsubscript{base}) &74.8&	71.5&	73.1&	82.1&	78.7&	80.4&	72.8&	69.6&	71.1&	69.3	&66.3&	67.8&	28.1&	95.4&	43.4\\
%         +BiLSTM &73.6&	70.8&	72.1&	81.2&	80.5&	80.8&	71.1&	72.1&	71.6&	68.6&	59.8&	63.9&	25.4&	95.5&	40.1\\
         % +BiLSTM &74.75&	71.5&	73.09	&82.14&	78.69&	80.38&	72.79&	69.55&	71.14&	69.31&	66.26&	67.75&	28.07&	95.38&	43.38\\
%         -Overlap &72.4	&71.2&	71.7&	80.1&	80.7&	80.4&	69.3&	72.6&	70.9&	67.8	&60.1	&63.7&	25.5&	96.0&	40.3\\
%         -Overlap+BiLSTM &74.1&	70.9&	72.3&	81.3&	80.8	&81.1&	71.4&	72.2&	71.8&	69.5&	59.6&	64.2&	25.5&	95.7	&40.2\\

%         Boundary(T5\textsubscript{base}) &67.6&	67.6&	67.5&	74.7&	76.3&	75.5&	62.7&	67.4&	65.0&	65.5&	59.1&	62.1&	25.0&	96.3&	39.7\\
%         +BiLSTM & 74.3&	69.7&	71.8&	82.1&	80.2&	81.1&	71.0&	70.3&	70.6&	69.7&	58.6&	63.7&	25.8&	97.0&	40.7\\
%         -Overlap&71.6	&69.7	&70.5&	79.5&	79.8&	79.6&	67.4&	70.5&	68.9&	67.8	&58.7&	62.9&	25.8&	96.9&	40.7\\
%         -Overlap+BiLSTM &72.9	&70.6	&71.6&	80.5&	80.9&	80.7&	68.9&	71.6&	70.2&	69.3&	59.2&	63.8&	25.8&	97.0&	40.8\\

%       \midrule
%         Enumeration(RoBERTa\textsubscript{base})  &71.2&	67.2&	69.1&	77.6&	75.6&	76.6&	68.6&	66.0&	67.3&	67.4&	59.9&	63.5&	25.0&	96.4&	39.7\\
        
%         +BiLSTM &71.8&	67.1	&69.3	&78.1	&75.7	&76.9	&68.9&	66.0&	67.4&	68.3&	59.6&	63.6&	24.9&	95.9&	39.5\\
        
%         -Overlap &73.91&	71.2	&72.5&	81.0&	81.0&	81.0&	71.4&	72.4&	71.9&	69.3&	60.3&	64.5&	25.5	&96.1	&40.4\\
        
%         -Overlap+BiLSTM& 74.5&	70.6&	72.4&	81.8&	80.6&	81.2&	72.0	&72.1&	72.0&	69.8&	59.1&	64.0&	25.5&	96.0&	40.3\\

%         Enumeration(T5\textsubscript{base})& 67.2&	67.2&	67.1&	74.3&	76.2&	75.2&	61.9&	66.9&	64.3&	65.3&	58.5&	61.7&	25.0&	96.3&	39.7\\
%         +BiLSTM &71.1	&66.9	&68.9	&78.1&	75.4&	76.7	&68.1&	65.5&	66.7&	67.1&	59.8&	63.3	&25.1&	96.5&	39.8\\
%         -Overlap &72.3	&68.7	&70.4&	80.3&	79.1&	79.7&	68.7&	69.0&	68.8&	67.9&	58.1	&62.6&	25.6&	96.4&	40.5\\
%         -Overlap+BiLSTM &71.5&	71.0&	71.3&	79.5&	78.4&	78.9&	67.7&	69.7&	68.7&	67.4	&64.9	&66.1&	28.2&	95.8&	43.6\\
%       \bottomrule
%     \end{tabular}
%     }
%     \caption{Full experiment results of coreference resolution task on CoNLL-12 dataset}
%     \label{tab:coref_baseline_exps}
%\end{table*}


% \subsection{Hyperparameter}
% \paragraph{OneIE}


% \paragraph{Coreference Resolution}

% \paragraph{Question Answering}
