# Supplementary material for: An Empirical Study on Finding Spans
Source: arXiv:2210.06824 source file (2022-10-14)
Supplement: Supplementary file 4 [file mention_breakdowns.tex]

 % This is the breakdown for the mention scores of OneIE, I am not sure where to add the table as well
 % I included entity mention and event mention(triggers)
 % Reminder: We used the model that without the additional typing layer as our baseline
\begin{table*}[h]
\resizebox{\linewidth}{!}{%
    \centering
    \begin{tabular}{l|cccccccccccc}
       \toprule
        \bf Approach & \multicolumn{3}{c}{\bf Entity-I} & \multicolumn{3}{c}{\bf Entity-C} & \multicolumn{3}{c}{\bf Trigger-I}& \multicolumn{3}{c}{\bf Trigger-C}\\
        \cmidrule(lr){2-4}\cmidrule(lr){5-7}\cmidrule(lr){8-10}\cmidrule(lr){11-13}
         & Prec & Rec & \bf F\textsubscript{1}& Prec & Rec & \bf F\textsubscript{1}& Prec & Rec & \bf F\textsubscript{1} & Prec & Rec & \bf F\textsubscript{1}\\
        \midrule
        Tagging (RoBERTa\textsubscript{base}) & 94.5 & 94.8 & 94.6 & 89.9 & 90.1 & 90.0 & 70.9 & 76.0 & 73.3 & 65.5 & 72.7 & 68.9\\
        Tagging (T5\textsubscript{base}) & 93.9 & 95.0 & 94.5 & 90.7 & 89.0 & 88.6 & 71 & 52.6 & 60.2 & 46.6 & 33.7 & 39.0\\
        \midrule
        Boundary Prediction (RoBERTa\textsubscript{base}) & 94.9 & 94.9 & 94.9 & 90.1 & 89.6 & 89.9 & 71.4 & 73.3 & 72.3 & 67.2 & 68.2 & 67.7 \\
        Boundary Prediction (T5\textsubscript{base}) & 95.6 & 95.4 & 95.5 & 90.7 & 90.3 & 90.5 & 69.4 & 72.0 & 70.7 & 67.5 & 69.3 & 68.3\\
        \midrule
        Span Enumeration (RoBERTa\textsubscript{base}) & 94.1 & 95.4 & 94.8 & 89.3 & 90.2 & 89.7 & 65.9 & 81.0 & 72.7 &62.5 &77.1 & 69.0\\
        Span Enumeration (T5\textsubscript{base}) & 88.6 & 95.6 & 92.0 & 83.1 & 89.6 & 86.2 & 45.1 & 86.2 & 59.2 & 36.4 & 69.5 & 47.8 \\
        \bottomrule
    \end{tabular}
    }
    \caption{Breakdowns for the mention scores.}
    \label{tab:mention_breakdown}
\end{table*}
